# Supplementary material for: Diffusion piecewise exponential models for survival extrapolation using Piecewise Deterministic Monte Carlo
Source: arXiv:2505.05932 source file (2025-05-09)
Supplement: Supplementary file 1 [file Supplementary_material.pdf]

# Supplementary materials for Diffusion piecewise exponential models for survival extrapolation using Piecewise Deterministic Monte Carlo

Luke Hardcastle*, Samuel Livingstone* and Gianluca Baio*

# 1 Additional modelling details

## 1.1 Derivation of the Gompertz drift

The Gompertz hazard function is given by $h_0(y) = \psi_1 \exp(\psi_2 y)$. Following (Roberts and Sangalli, 2010) we assume this is the solution to an autonomous differential equation

$$\begin{aligned}\frac{dh_0(y)}{dy} &= g(h_0(y)) \\ &= \psi_1\psi_2 \exp(\psi_2 y) \\ &= \psi_2 h_0(y).\end{aligned}$$

This can then be transformed to the log-scale via a change of variables to arrive at the required drift

$$\begin{aligned}h_1(y) &= \log(h_0(y)), \\ \frac{dh_1(y)}{dh_0(y)} &= \frac{1}{h_0(y)}\psi_1 h_0(y) = \psi_1 = \mu(\alpha_y).\end{aligned}$$

## 1.2 Penalised-complexity prior derivation

We place a penalised complexity prior (Simpson et al., 2017) on the step size, $\sigma$, corresponding to the prior

$$\sigma \sim \text{Exponential}(a).$$

Following the reasoning presented in Simpson et al. (2017) we calibrate $a$ through the probability

$$\mathbb{P}(\sigma > U) = \alpha.$$

Given the discretised diffusion prior presented in Section 2, this prior should place the majority of its mass $< 1$ to preserve the numerical stability of the skew-symmetric discretisation scheme (Livingstone et al., 2024). Setting $a = 2$ gives

$$\mathbb{P}(\sigma > 1) = 0.135,$$

suggesting this is appropriately penalising $\sigma$. Following the reasoning of (Simpson et al., 2017) we expect this prior to be relatively insensitive to the specification of $a$.

---

arXiv: 2010.00000

*Department of Statistical Science, University College London, luke.hardcastle.20@ucl.ac.uk; samuel.livingstone@ucl.ac.uk; g.baio@ucl.ac.uk

# 2 Additional computational details

## 2.1 Algorithms

The core loop of the sampling algorithm consists of two components *i)* Generating the sticky PDMP dynamics for a fixed set of candidate knots $\{m_i\}_{i=1}^M$. *ii)* Updating the set of candidate knots and (if required) the hyperparameter $\gamma$. The former can be achieved using either Algorithm 1 or Algorithm 2. The latter is specified in Algorithm 3. Note that the method provided in Algorithm 1 is inexact without a Metropolis correction, with the induced bias vanishing as $\delta \to 0$ (Bertazzi et al., 2023). This can be added after each loop of the algorithm. The results in the main paper are generated using the uncorrected version of Algorithm 1. The updates to $v^{\nabla U}, v^{\perp}$ are given by the positive p-orthogonal refresh forward event chain Monte Carlo method of (Michel et al., 2020).

**Algorithm 1** Generating the PDMP via splitting schemes

Given step size $\Delta t$, current state $z_0 = (x_0, v_0)$ and current $b$
Simulate $U_1, U_2, U_3 \overset{iid}{\sim} \text{Uniform}(0, 1)$
**if** $U_1 < 1 - \exp(-\lambda_e \Delta t/2)$ **then**
    Set $b = 1$
**end if**
Update $x_0 \mapsto x_{\Delta t/2}$, ▷ Sticky PDMP dynamics
**if** $U_2 < 1 - \exp(-\lambda(\Delta t/2)\Delta t)$ **then**
    **if** $b = 0$ **then**
        Update $v^{\nabla U}$
    **end if**
    **if** $b = 1$ **then**
        Update $v^{\nabla U}, v^{\perp}$
        Set $b = 0$
    **end if**
**end if**
Update $x_{\Delta t/2} \mapsto x_{\Delta t}$.
**if** $U_3 < 1 - \exp(-\lambda_e \Delta t/2)$ **then**
    Set $b = 1$
**end if**

**Algorithm 2** Generating the PDMP using Gibbs updates and line search

Given current $z_0 = (x_0, v_0)$, $\sigma_0$.
Simulate $t_h \sim \text{Exponential}(\lambda_h)$.
Update $z_0 \mapsto z_{t_h}$ ▷ Sticky PDMP dynamics via (Bouchard-Côté et al., 2018, Example 1)
Sample $\sigma$ from the full conditional $\pi(\sigma \mid z_{t_h})$. ▷ Metropolis-within-Gibbs

**Algorithm 3** Updating $\{m_i\}_{i=1}^M$ and $\Gamma$

1: Given $z_t, \Gamma_t, \{s_j\}_{j=1}^J, \{m_i\}_{i=1}^M$.
2: Update $z_t, \{s_j\}_{j=1}^J$ ▷ Algorithm 1 or Algorithm 2
3: Update $K = M - J$, $K \sim \text{Poisson}((1-\omega)\Gamma y_+)$
4: Update $\{r_j\}_{j=1}^{M-J} \overset{iid}{\sim} \text{Uniform}(0, y_+)$
5: Update $\Gamma \sim \text{Gamma}(J + \alpha, \omega/(\beta + 1))$ ▷ If hyperprior specified

## 2.2 Generating extrapolations

In Section 3.6 we highlight that extrapolations can: *i)* Be generated using the skew-symmetric scheme directly. This reduces the computational cost of the methods. *ii)* Be generated using a re-scaled consistent step size $\sigma^*$. This gives the practitioner more control over the computational cost of generating extrapolations, and the bias induced by using a discretisation scheme. Given $\sigma^*$, extrapolations can be generated using a set of times with inter-arrival times given by

$$\{\tau_i\}_{i=1}^N \overset{iid}{\sim} \text{Exponential}(\Gamma\omega(\sigma/\sigma^*)^2).$$

In the examples of Section 4 we use $\sigma^* = 0.1$.

## 2.3 Reversible jump MCMC

The reversible jump algorithm of Section 3.7 alternates between a random walk Metropolis update to $\tilde{\theta}$ and reversible jump moves which add and delete knots in the samplers (Green, 1995). Knots are added as

1. Propose a new knot location $s_j^* \sim \text{Uniform}(s_1, y_+)$.

2. Propose a new value for the scaled innovation at that knot, $\tilde{\theta}_j^* \sim \text{Normal}(0, \sigma_{RJ}^2)$.

3. Accept the proposed knot and innovation with probability $\min\{1, A\}$ with

$$A = \frac{\pi(\tilde{\theta}^*, s^*)/(J+1)}{\pi(\tilde{\theta}, s)q(\tilde{\theta}^*)}.$$

   Where $q(\cdot)$ is the proposal density, and the $J+1$ term arises as the probability of picking a knot to remove in the reverse move.

Knots are removed by selecting a knot and corresponding innovation to remove from the model. These moves are accepted with probability $\min\{1, A^{-1}\}$.

The reversible jump sampler in Section 3.7 was run using a step size of 0.05 for the Random Walk Metropolis kernel and 0.01 for the step size of the reversible jump proposal. The sampler was run for 1,000,000 iterations, with one iteration consisting of a single Random Walk Metropolis and reversible jump step. The PDMP sampler was

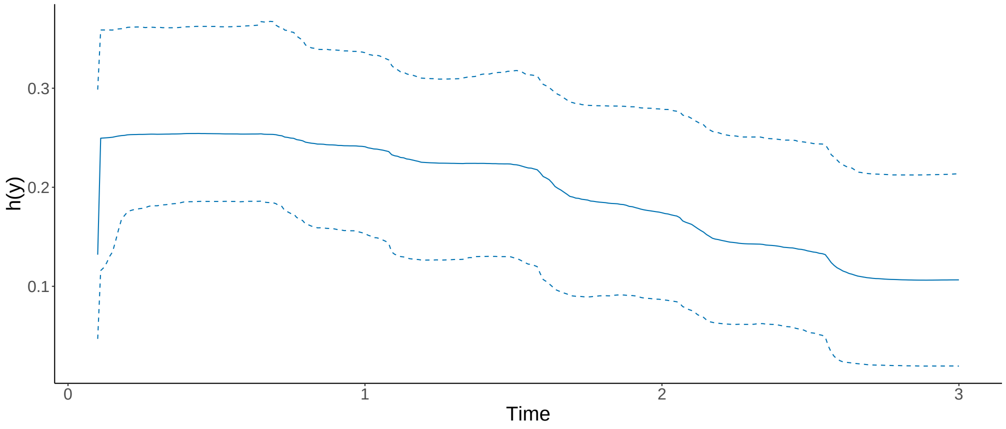


Figure 1: Hazards under the reversible jump sampler with alternative reversible jump proposal parameter.

run for the same computational budget. Using a step size of 1 in the reversible jump proposal results in the hazards in Figure 1.

We also sought to compare the sampler developed in Section 3 to an existing sampler. To this end the results of applying the piecewise exponential model of (Chapple et al., 2020) to the Colon cancer. The resulting hazard is plotted in Figure 2. In this case both the reversible jump and within model sampling components have failed to explore the state space. This serves to illustrate the difficulty in designing and implementing these samplers.

# 3 Additional details for example applications

All the models were implemented in Julia with code available at `https://github.com/LkHardcastle/PEM_extrap`.

## 3.1 Specification of $\gamma$

To find the optimal value of $\gamma$ models were fit to the Colon cancer data using $\mu(\alpha_j) = 0$, for $\Gamma \in \{1, 2, 5, 10, 15, 20, 25\}$. LOOIC values were computed using Pareto-smoothed importance sampling (Vehtari et al., 2017). These values are plotted in Figure 6. While the LOOIC decreases as $\gamma$ increases, the improvement begins to plateau between $\Gamma = 5$ and $\Gamma = 10$, indicating $\Gamma = 7$ as a good choice of hyperparameter.

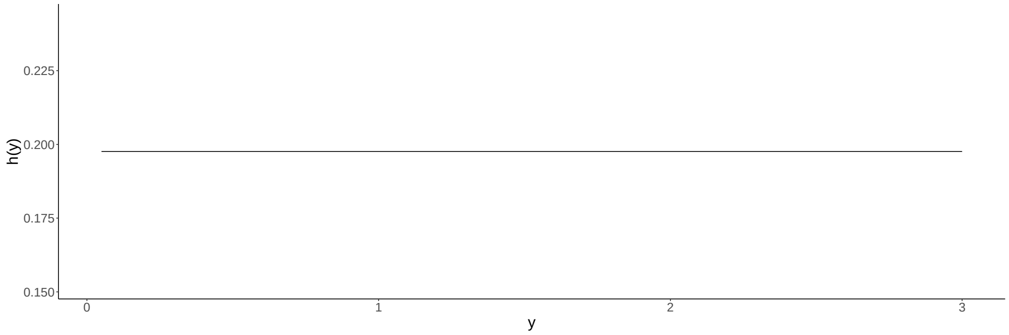


Figure 2: The mean hazard under the piecewise exponential model and sampler of Chapple et al. (2020).

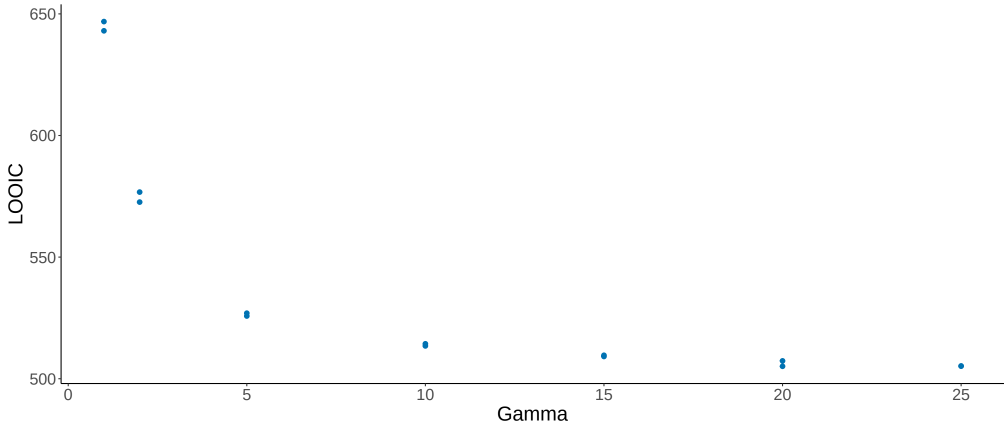


Figure 3: LOOIC values for various values of $\Gamma$ for the colon cancer data.

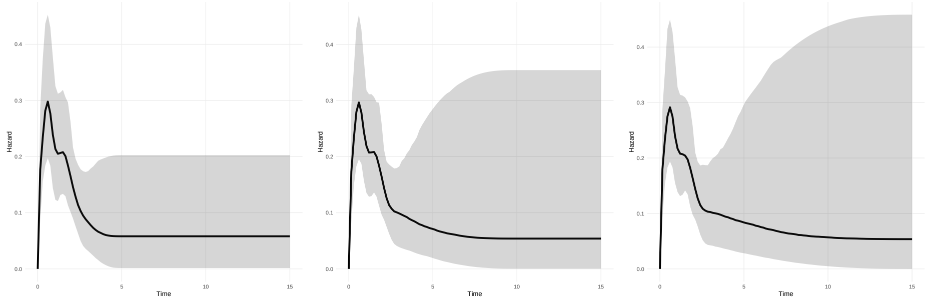


Figure 4: Hazards for the M-spline hazard model fit to the Colon cancer data with the final knot placed at 5, 10 and 15 years (Jackson, 2023). Note how extrapolations are strongly dependent on the placement of the final knot.

## 3.2 Colon cancer data

The Colon cancer data were accessed via the `R` `survextrap` package. Each model was run for 2 chains of 10,000 iterations, 5,000 of which were burn-in, and where each iteration consists of a single Gibbs update for $\{r_k\}_{k=1}^{M-J}$ and 50 iterations of Algorithm 1 with $\Delta t = 0.01$ Convergence was assessed by examining trace plots, $\hat{R}$ values for the hazard at fixed time points and effective sample sizes. Priors were as specified in Sections 2 and Section 4.1. The specific drift functions were derived as follows. The log-Gamma(2,7) stationary distribution was elicited by assuming a constant (exponential) hazard as $y \to y_\infty$. Using standard conjugacy results this can be elicited by assuming the observation of $a$ individuals for $b$ time until events was observed. This stationary prior implies 2 individuals observed for a total of 7 years in the limit. The Gaussian Langevin stationary distribution was then selected to approximately match the uncertainty intervals of this Gamma distribution. We note that these examples are purely illustrative and can likely be improved on in practice.

## 3.3 Comparators

Figure 4 and Figure 5 show hazard functions for the comparators in Section 4.1 (Baio, 2020; Cooney and White, 2023; Jackson et al., 2017). The results for the standard parametric models are presented in Table 1. AIC is minimised for the log-normal model, and as such this is the model used as the comparator in the main manuscript.

## 3.4 CLL-8 trial data

The same procedure as for the Colon cancer data was used to determine an optimal value of $\Gamma$. The results of this procedure are shown in Figure 6. While the LOOIC is minimised for $\Gamma = 20$, the values begin to plateau around $\Gamma = 10$. Each model was run for 2 chains of 10,000 iterations, 5,000 of which were burn-in, and where each iteration consists of a single Gibbs update for $\{r_k\}_{k=1}^{M-J}$ and 50 iterations of Algorithm 1 with

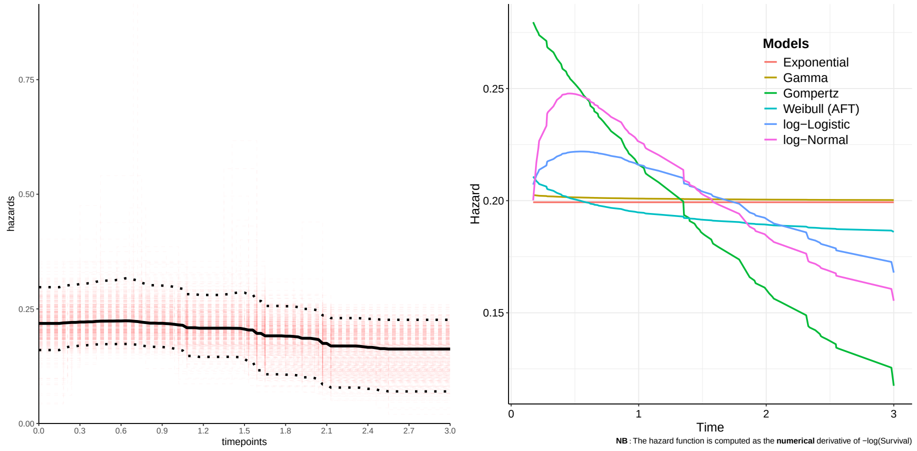


Figure 5: (Left) Hazards for the independent piecewise exponential model fit to the Colon cancer data (Cooney and White, 2023). Note how the hazard is not as expressive as either the diffusion piecewise exponential model or the M-spline model. (Right) Hazards for the standard parametric models fit to the colon cancer data. Hazards are computed using numerical derivatives of $-\log(S(y))$ and as such appear non-smooth in the plot.

| Model | AIC | $\mathbb{E}[Y](0, y_+)$ | $\mathbb{E}[Y](0, y_\infty)$ |
|---|---|---|---|
| Exponential | 431.57 | 2.22 (2.06, 2.35) | 4.71 (3.80, 5.63) |
| Gamma | 433.56 | 2.21 (2.08, 2.35) | 4.73 (3.73, 5.72) |
| Gompertz | 428.20 | 2.15 (1.98, 2.30) | 7.12 (4.70, 8.75) |
| Weibull | 433.34 | 2.20 (2.05, 2.35) | 4.89 (3.78, 5.96) |
| Log-logistic | 428.24 | 2.18 (2.02, 2.32) | 5.60 (4.57, 6.61) |
| Log-normal | 422.19 | 2.18 (2.03, 2.32) | 5.79 (4.71, 6.86) |

Table 1: Results for the standard parametric models fit to the Colon cancer data. Mean survival results and 95% confidence intervals are reported.

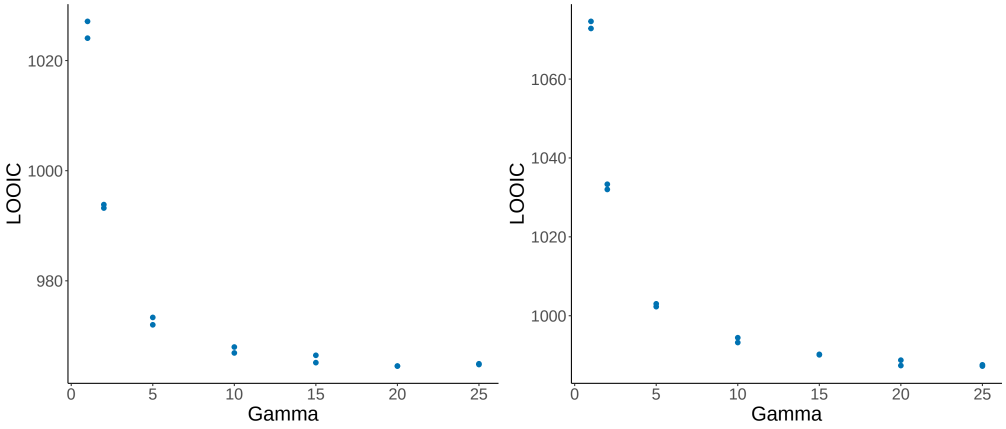


Figure 6: LOOIC values for various values of $\Gamma$ for the CLL-8 data.

$\Delta t = 0.01$ Convergence was assessed by examining trace plots, $\hat{R}$ values for the hazard at fixed time points and effective sample sizes.

We outline the time-varying drift functions used in Section 4.2.

**Gamma waning:**

$$\mu(\alpha_y, y) = \psi_1(y) - \psi_2(y)\exp(\alpha_y),$$
$$\psi_1(y) = \psi_1 \max\{\min\{1, y/c\}, 1/c\}, \quad \psi_2(y) = \psi_2 \max\{\min\{1, y/c\}, 1/c\}.$$

**Waning treatment effect:**

$$\mu(\beta_y, y) = \frac{1}{\psi_2(y)^2}\beta_y, \quad \psi_2(y) = \max(1, (y/4)^2)^{-1}.$$

## References

Baio, G. (2020). "survHE: survival analysis for health economic evaluation and cost-effectiveness modeling." *Journal of Statistical Software*, 95: 1–47. 6

Bertazzi, A., Dobson, P., and Monmarché, P. (2023). "Piecewise deterministic sampling with splitting schemes." *arXiv preprint arXiv:2301.02537*. 2

Bouchard-Côté, A., Vollmer, S. J., and Doucet, A. (2018). "The bouncy particle sampler: A nonreversible rejection-free Markov chain Monte Carlo method." *Journal of the American Statistical Association*, 113(522): 855–867. 2

Chapple, A. G., Peak, T., and Hemal, A. (2020). "A novel Bayesian continuous piecewise linear log-hazard model, with estimation and inference via reversible jump Markov chain Monte Carlo." *Statistics in medicine*, 39(12): 1766–1780. 4, 5

Cooney, P. and White, A. (2023). "Extending Beyond Bagust and Beale: Fully Parametric Piecewise Exponential Models for Extrapolation of Survival Outcomes in Health Technology Assessment." *Value in Health*, 26(10): 1510–1517. 6, 7

Green, P. J. (1995). "Reversible jump Markov chain Monte Carlo computation and Bayesian model determination." *Biometrika*, 82(4): 711–732. 3

Jackson, C., Stevens, J., Ren, S., Latimer, N., Bojke, L., Manca, A., and Sharples, L. (2017). "Extrapolating Survival from Randomized Trials Using External Data: A Review of Methods." *Medical Decision Making*, 37(4): 377–390. PMID: 27005519. 6

Jackson, C. H. (2023). "survextrap: a package for flexible and transparent survival extrapolation." *BMC Medical Research Methodology*, 23(1): 282. 6

Livingstone, S., Nüsken, N., Vasdekis, G., and Zhang, R.-Y. (2024). "Skew-symmetric schemes for stochastic differential equations with non-Lipschitz drift: an unadjusted Barker algorithm." *arXiv preprint arXiv:2405.14373*. 1

Michel, M., Durmus, A., and Sénécal, S. (2020). "Forward event-chain Monte Carlo: Fast sampling by randomness control in irreversible Markov chains." *Journal of Computational and Graphical Statistics*, 29(4): 689–702. 2

Roberts, G. O. and Sangalli, L. M. (2010). "Latent diffusion models for survival analysis." *Bernoulli*, 16(2): 435 – 458. 1

Simpson, D., Rue, H., Riebler, A., Martins, T. G., and Sørbye, S. H. (2017). "Penalising Model Component Complexity: A Principled, Practical Approach to Constructing Priors." *Statistical Science*, 32(1): 1 – 28. 1

Vehtari, A., Gelman, A., and Gabry, J. (2017). "Practical Bayesian model evaluation using leave-one-out cross-validation and WAIC." *Statistics and computing*, 27: 1413–1432. 4
